# Supplementary material for: Quantum Coulomb Liquids of Different Rank in the Breathing Pyrochlore Antiferromagnet
Source: arXiv:2602.15662 source file (2026-02-17)
Supplement: Supplementary file 1 [file Rank_2_BreathingPyro_DM_SM.pdf]

# Supplemental Material for
# "Quantum Coulomb Liquids of Different Rank in the Breathing Pyrochlore Antiferromagnet"

Lasse Gresista,[1,2,*] Daniel Lozano-Gómez,[3,*] Matthias Vojta,[3] Simon Trebst,[1] and Yasir Iqbal[2]

[1]*Institute for Theoretical Physics, University of Cologne, 50937 Cologne, Germany*
[2]*Department of Physics and Quantum Center for Diamond and Emergent Materials (QuCenDiEM), Indian Institute of Technology Madras, Chennai 600036, India*
[3]*Institut für Theoretische Physik and Würzburg-Dresden Cluster of Excellence ctd.qmat, Technische Universität Dresden, 01062 Dresden, Germany*

(Dated: February 17, 2026)

## BAND EVOLUTION

As discussed in the main text, the quantum model describing the breathing pyrochlore lattice realizes two additional non-conventional phases that are not realized in the classical model, namely the PM and the ICS phase. In the classical model, previous works [1–3] have associated the realization of a non-conventional phase with the observation of energy-minima in the lowest energy band of the interaction matrix $J^{\alpha\beta}(\boldsymbol{q})$ away from the $\Gamma$ point. As a first approach and to assess the possibility of realizing a non-conventional magnetically ordered phase in the classical model, we study the interaction matrix $J^{\alpha\beta}(\boldsymbol{q})$ energy bands in regions in parameter space where the PM and ICS phases are observed in the quatum model. Figure S1 illustrates the energy bands for five distinct sets of parameters along a high-symmetry path in reciprocal space. For all the sets of parameters we considered, the lowest energy band has a minimum at the $\Gamma$ point, suggesting that the low-temperature phase is given by a $\boldsymbol{q} = 0$ ordered phase. This claim is further supported by our classical Monte Carlo simulations where a $\Gamma_5$ phase is identified as the low-temperature phase for sets of interaction parameter away from the $D_b = 0$ $(D_a = 0)$ line.

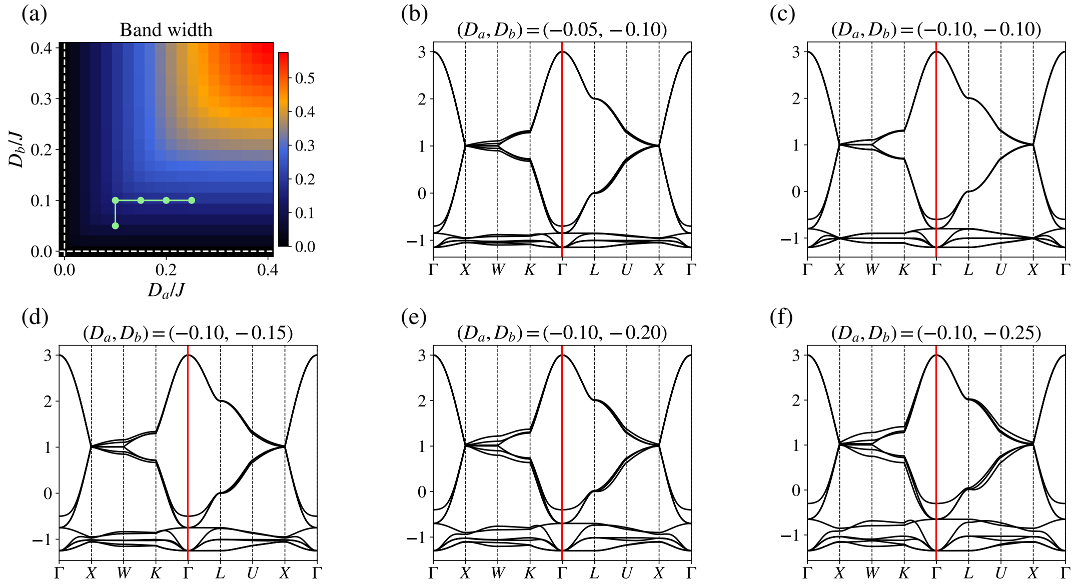


FIG. S1. **Parametric dependence of energy bands of the classical model**. (a) Evolution of the band width of the lowest-energy band of the interaction matrix $J^{\alpha\beta}(\boldsymbol{q})$ as a function of the interaction parameters $D_a$ and $D_b$. The white dashed lines mark the cases $D_b = 0$ $(D_a = 0)$ where the lowest-energy band is completely flat. (b-f) Interaction-matrix $J^{\alpha\beta}(\boldsymbol{q})$ bands along a high-symmetry path in reciprocal space for five distinct sets of parameters $D_a$ and $D_b$ indicated in above each panel. The red vertical line marks the $\Gamma$ point whenever the lowest-energy band presents a global minimum at that wave vector. In panel (a) the green dots mark the precise location of the interaction parameters used to produce panels (b)-(f).

## ADDITIONAL MOMENTUM-SPACE CUTS OF THE STRUCTURE FACTOR

In the main text, we present neutron-scattering structure factors in selected high-symmetry planes of momentum space that most clearly highlight the characteristic pinch-point and ordering features of the different phases. For completeness, in Fig. S2

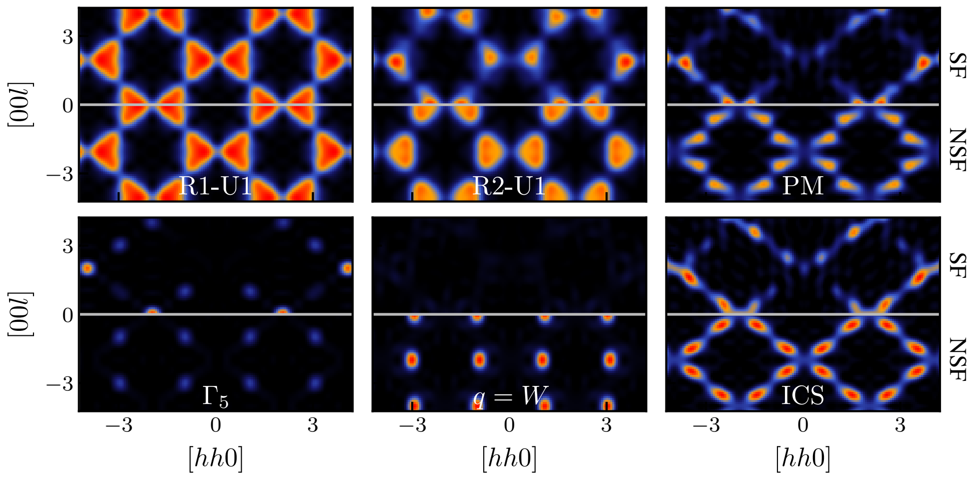


FIG. S2. **Structure factors in the hhl plane from pf-FRG.** Polarized neutron scattering structure factors in the spin-flip (SF, top) and non-spin-flip (NSF, bottom) channels in the $hhl$ plane for each phase, calculated in the low-cutoff limit.

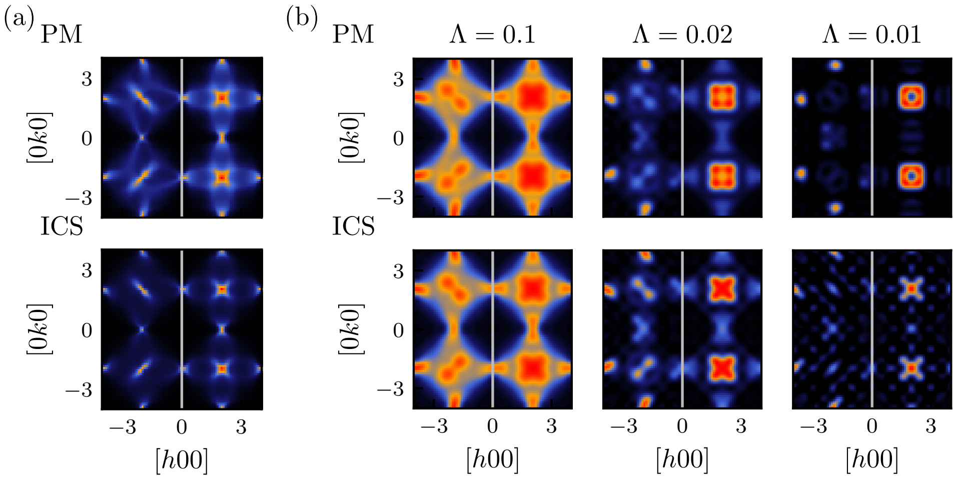


FIG. S3. **Structure factors in the PM and ICS phase in the hk0-plane from pf-FRG.** (a) Neutron-scattering structure factor obtained from SCGA in the cooporative paramagnetic regimes at $T > T_c$ for characteristic points where the pf-FRG identifies the PM and ICS phases. The left (right) side show the spin-flip (non–spin-flip) channel. (b) Corresponding neutron-scattering structure factor obtained from pf-FRG at different RG cutoff scales $\Lambda$.

we additionally show the corresponding polarized structure factors in the $hhl$ plane for all phases in the low-cutoff limit. Furthermore, Fig. S3 displays the evolution of the structure factor in the $hk0$ plane across the PM and ICS regimes, comparing classical SCGA results above $T_c$ with quantum pf-FRG data at different RG cutoffs $\Lambda$.

## SELF-CONSISTENT GAUSSIAN APPROXIMATION

In this section, we provide a brief overview of the self-consistent Gaussian approximation (SCGA) and how this approach can be used to obtain spin correlation functions and internal energy. This approximation, also known as large-$\mathcal{N}$ approximation, replaces the hard constraint on the spin length, $|\boldsymbol{S}_i|^2 = S^2$, by a soft (average) spin-length constraint, i.e. $\langle|\boldsymbol{S}_i|^2\rangle = S^2$. The soft spin-length constraint is fulfilled by the introduction of a Lagrange multiplier $\lambda$. This approximation results in a quadratic (Gaussian) theory which can be exactly solved [4–6] to obtain various quantities of interest.

For this approximation, we consider a general bilinear anisotropic spin Hamiltonian written in the form

$$\mathcal{H} = \frac{1}{2} \sum_{i\mu,j\nu} \sum_{\alpha,\gamma} S^{\alpha}_{i\mu} \, \boldsymbol{J}^{\alpha,\gamma}_{i\mu,j\nu} \, S^{\gamma}_{j\nu}, \tag{S1}$$

where the sub-indices $i$ and $j$ label the primitive vectors $\boldsymbol{R}_i$, while $\mu$ and $\nu$ denote a sublattice basis. For the (breathing)

pyrochlore lattice, the $\boldsymbol{R}_i$ vectors refer to FCC points, whereas the indices $\mu$ and $\nu$ labels the four sublattice sites of a tetrahedron. The Fourier space spin-spin correlation function, for $\alpha$ and $\gamma$ Cartesian spin components and for sublattices $\mu$ and $\nu$ takes the form

$$\mathcal{S}_{\mu\nu}^{\alpha\gamma} = \langle S_\mu^\alpha(\boldsymbol{q}) S_\nu^\gamma(-\boldsymbol{q})\rangle = (G_{\mu\nu}^{\alpha\gamma}(\boldsymbol{q}))^{-1} = (\beta \boldsymbol{J}_{\mu\nu}^{\alpha\gamma}(\boldsymbol{q}) + \lambda)^{-1}., \tag{S2}$$

where the Lagrange multiplier $\lambda$ is determined self-consistently as a function of temperature $T = 1/\beta$ by enforcing the soft spin-length constraint

$$S^2 = \frac{1}{N}\sum_{n,\boldsymbol{q}} (\beta\varepsilon_n(\boldsymbol{q}) + \lambda)^{-1}, \tag{S3}$$

where $\varepsilon_n(\boldsymbol{q})$ is the $n$-th eigenvalue of the interaction matrix $\boldsymbol{J}_{i\mu,j\nu}^{\alpha,\gamma}$ in Eq. (S1) expressed in momentum space (i.e., $\boldsymbol{J}_{\mu\nu}^{\alpha\gamma}(\boldsymbol{q})$), and $N$ is the number of lattice sites considered. Finally, though this approximation, the internal energy of the system is computed as

$$\mathcal{E} = \frac{1}{2N}\sum_{\boldsymbol{q}} \mathrm{Tr}\left[G(\boldsymbol{q})J(\boldsymbol{q})\right]. \tag{S4}$$

In the main text, we provide the prediction of the polarized neutron structure factors obtained via SCGA and classical Monte Carlo for a system along the $D_b = 0$ ($D_a = 0$) line, where excellent agreement is found *above* the transition temperature $T_c$ where the system undergoes a symmetry-breaking transition to a low-temperature $\boldsymbol{q} = \boldsymbol{W}$ phase. Furthermore, we find excellent agreement between the internal energy sampled via classical Monte Carlo and the behavior obtained via SCGA, see Fig. S4.

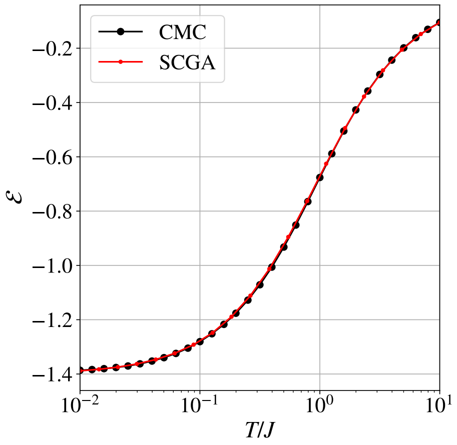


FIG. S4. **Internal energy.** Comparison between the internal energy sampled via classical Monte Carlo (CMC) and SCGA for a system along the $D_b = 0$ ($D_a = 0$) line.

It is, however, important to note that the symmetry-breaking transition cannot be captured by a quadratic theory, and therefore by SCGA. Moreover, and since the lowest-energy bands associated with this model are flat (see Fig. 2(b) of the main text), a SCGA theory predicts the realization of a classical spin-liquid phase down to the lowest temperatures, thus missing the symmetry-breaking transition.

* These authors contributed equally to the project.

[1] N. Francini, L. Janssen, and D. Lozano-Gómez, Higher-rank spin liquids and spin nematics from competing orders in pyrochlore magnets, Phys. Rev. B **111**, 085140 (2025).
[2] N. Francini, L. Schmidt, L. Janssen, and D. Lozano-Gómez, Exact nematic and mixed magnetic phases driven by competing orders on the pyrochlore lattice, (2025), arXiv:2510.23704.
[3] A. Itamar, Spin-Spin Correlations in the $CuAlCr_4S_8$ Breathing Pyrochlore, M.Sc. thesis, University of Waterloo, (2023).
[4] D. A. Garanin and B. Canals, Classical spin liquid: Exact solution for the infinite-component antiferromagnetic model on the kagomé lattice, Phys. Rev. B **59**, 443 (1999).
[5] B. Canals and D. A. Garanin, Spin-liquid phase in the pyrochlore anti-ferromagnet, Can. J. Phys. **79**, 1323 (2001).
[6] D. Lozano-Gómez, O. Benton, M. J. P. Gingras, and H. Yan, An Atlas of Classical Pyrochlore Spin Liquids, (2024), arXiv:2411.03547.
